# Supplementary material for: Impulse data models for the inverse problem of electrocardiography
Source: arXiv:2102.00570 source file (2021-08-19)
Supplement: Supplementary file 1 [file supplementarymaterial.tex]

\clearpage

\setcounter{figure}{0} 
\setcounter{equation}{0}
\textbf{Supplementary Materials}

\subsection{Body and Heart Surface 2D Projections}
We performed 2D geometry projections for the heart surface electrodes and body surface electrodes separately for each instance in time. At every instance in time, there are 108 HSP and 128 BSP electrode potential values. The heart surface electrodes were projected onto an evenly spaced 9-by-12 mesh as shown in Fig~\ref{fig:heartProj}. Using this heart 2D projection, the LV paced averaged beat HSP was projected into a 3D array of size 9-by-12-by-649. The body mesh from an experimental torso tank was used to project the body surface electrodes onto a cylinder approximation of the body using \textit{pointCloud} in MATLAB~\cite{Le2018}, as shown in Fig~\ref{fig:bodyProj}. The cylinder was unwrapped via a cut along the left anterior descending artery line identified in the experimental data. Bad leads identified via the experimental data were removed. The 2D unwrapped cylinder surface was re-sampled onto a 16-by-16 mesh via linear interpolation using \textit{griddata} in MATLAB. 

\begin{figure}[bth]
  \includegraphics[width=\columnwidth]{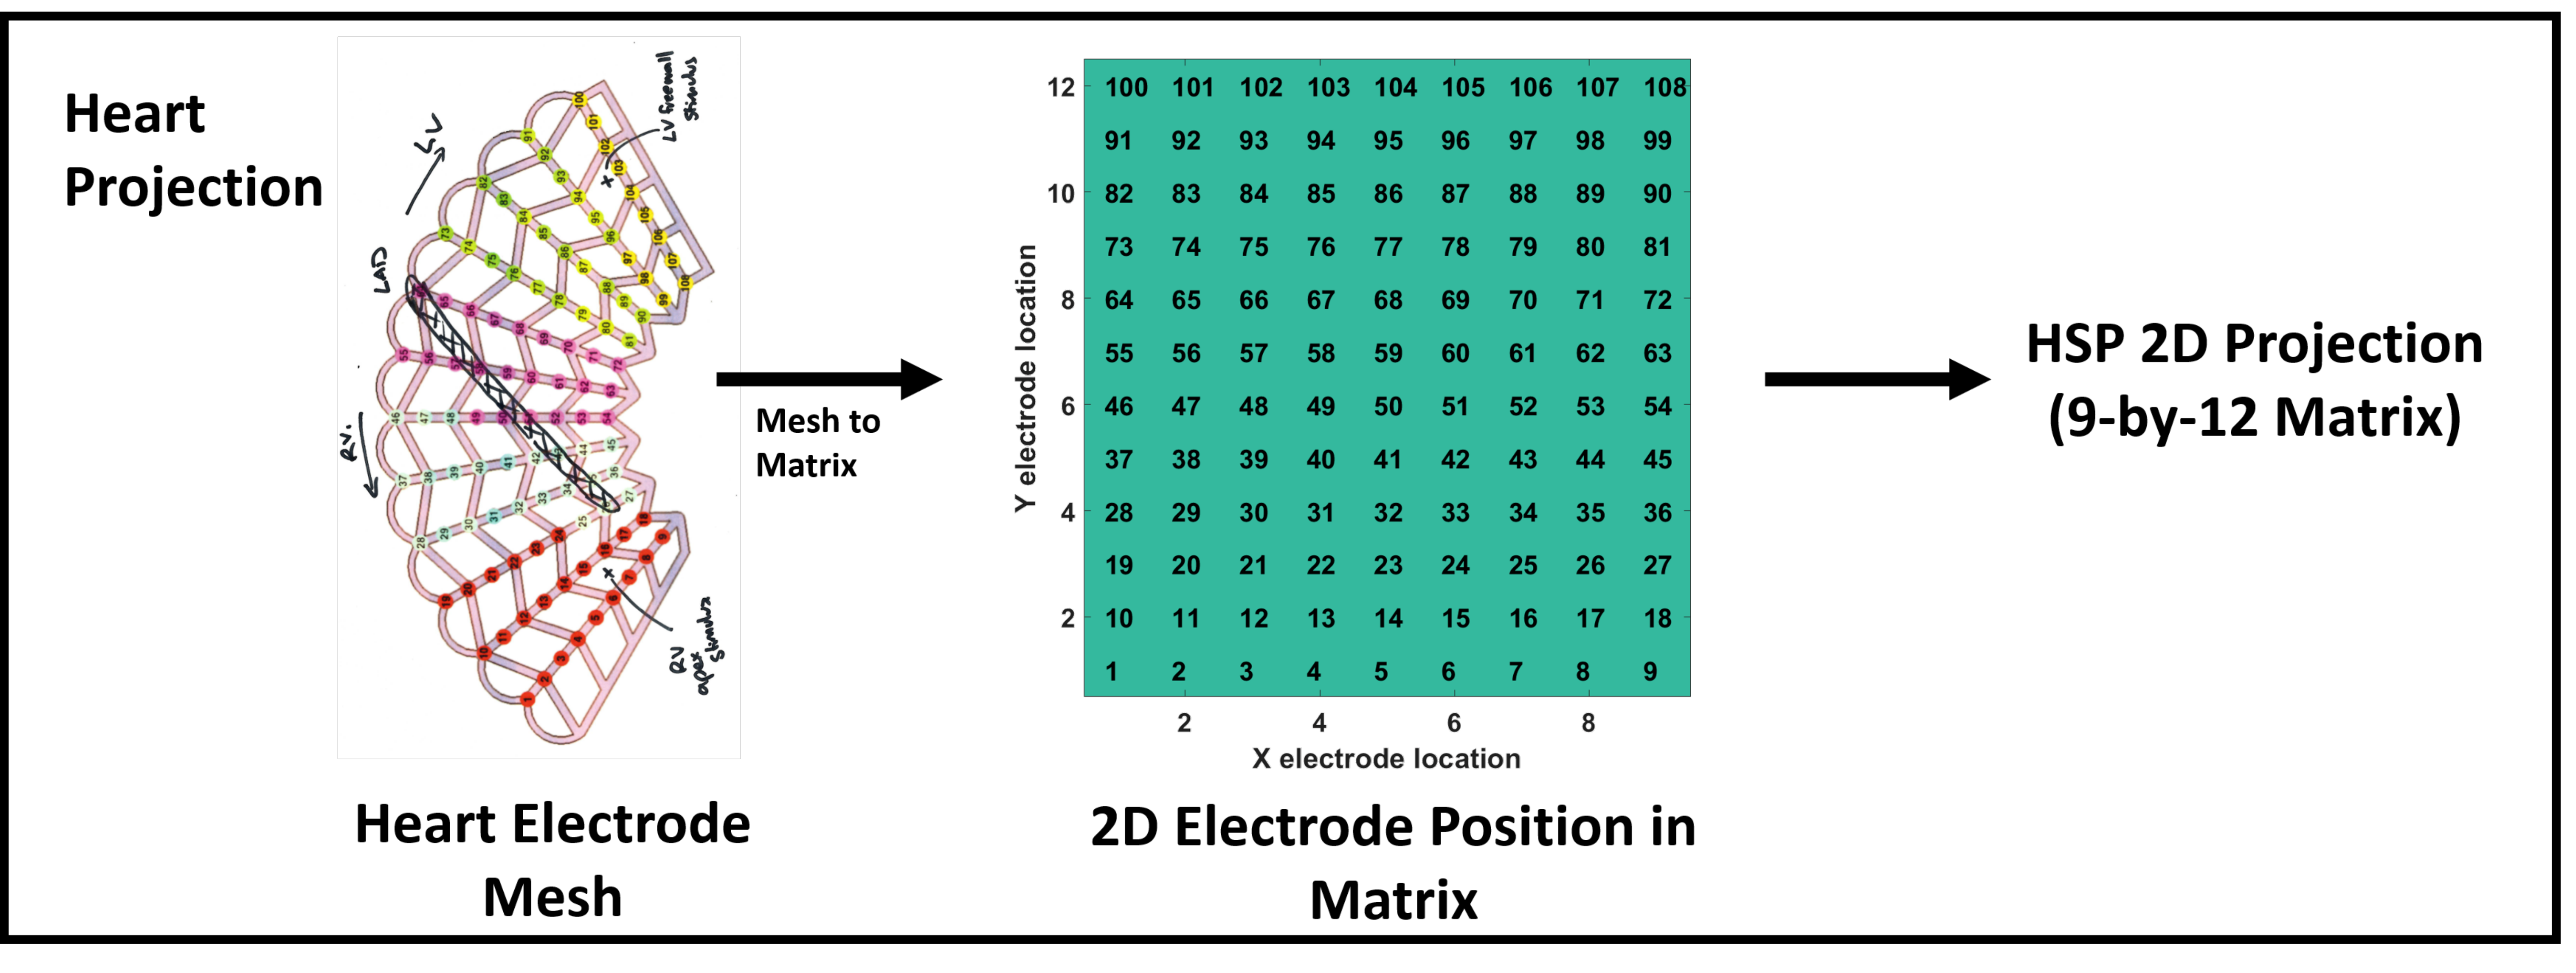}
  \caption{Summary of heart electrode 2D projection, where electrodes in a mesh were projected into 9-by-12 matrix positions.}
  \label{fig:heartProj}
\end{figure}

\begin{figure}[bth]
  \includegraphics[width=\columnwidth]{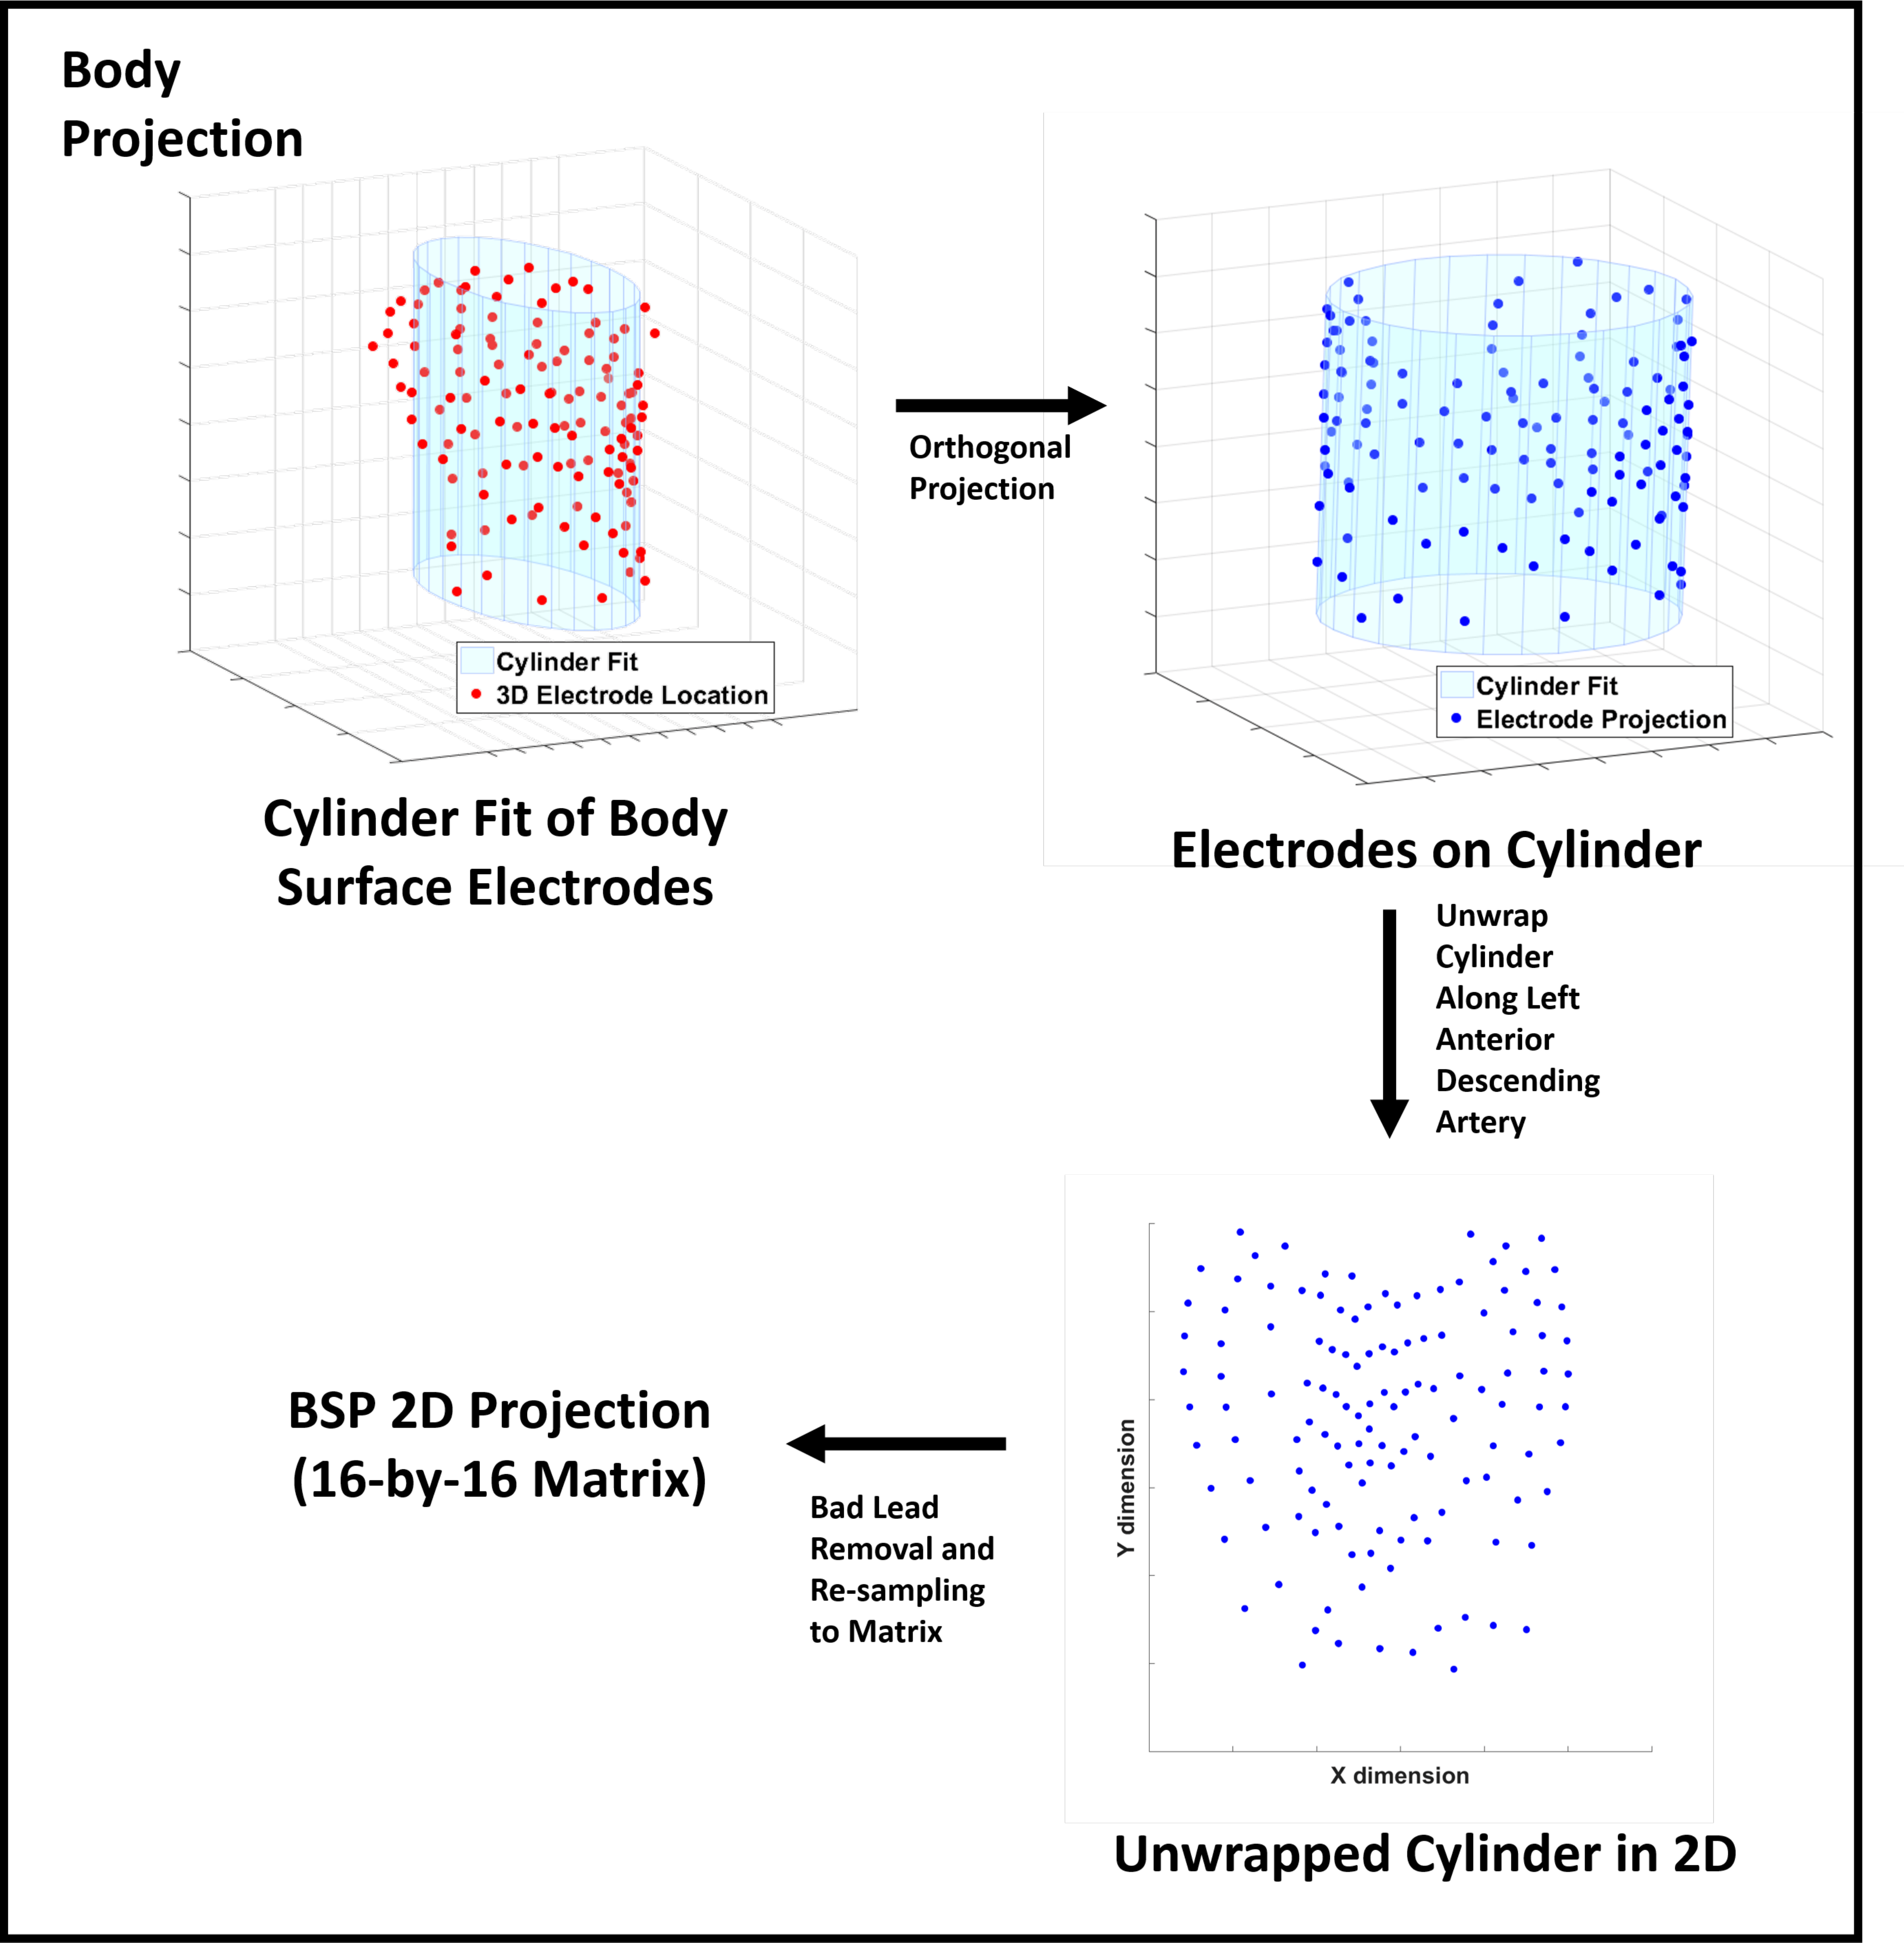}
  \caption{Summary of body electrode 2D projection. Electrodes in 3D space were first projected onto a cylinder. The cylinder was then unwrapped along the left anterior descending artery line. The unwrapped 2D surface was then re-sampled into 16-by-16 mesh positions.}
  \label{fig:bodyProj}
\end{figure}

This 16x16 body surface grid discretization is in dimensions of powers of 2, but reasonable. This is because many neural networks (such as convolutional neural networks) which take images as inputs perform well when presented with convolution filter windows of pixel size $2^{n}$ for each dimension (where $n$ is an integer). Therefore, the 16x16 mesh is the smallest mesh which fit this $2^n$ size requirement while also maintaining more mesh locations than the number of body surface electrodes ($>$128). Any smaller meshes (such as 8x8 = 64) would allow for fewer number of mesh points when compared to the number of BSP recording points. This essentially reduces the neural network input information to below that of the actual BSP recordings. Any larger meshes (such as 32x32 = 1024) would allow for fine representation of the unwrapped cylinder surface but require more interpolation of potential values. This essentially creates new values through informed guesses within this finer mesh.

\subsection{G3D Library}
A combination of different G3D parameters were used to create a G3D library which can describe a wide range of signal shapes and sizes. Here, the G3D basis functions within the library all have $\mathcal{A}=1$. The $\mu_{x}$ was allowed to vary in 8 even locations between 1 and 9 (9 is the size of the x dimension for signal to be fitted). The $\mu_{y}$ was allowed to vary in 8 even locations between 1 and 12 (12 is the size of the y dimension for signal to be fitted). The $\mu_{t}$ was allowed to vary evenly in 2, 4, 8, 16, 32, 64 splits between 0 and 1 ($t$ has units in heart beat time, varies between 0 and 1). The $\sigma_{xy}$ was allowed to vary evenly in 2, 4, 8, 16, 32, 64 splits between 0 and 0.5. The $\sigma_{t}$ was allowed to vary evenly in 2, 4, 8, 16, 32, 64 splits between 0 and 1. The final G3D library contained G3D basis functions generated from all given combinations of the 6 parameters.

\subsection{Predictions of Other Pacing Scenarios}
HSP activation maps were predicted from sinus rhythm (SR), bi-ventricular (BiV), and right ventricular (RV) pacing scenarios made under the same recording conditions (Fig~\ref{fig:realworldothercombo}). ECGI predicted activation times were also found and are shown in Fig~\ref{fig:realworldothercombo}. The mean absolute difference in activation times across all electrodes for impulse predictions is $8.06\pm8.03$ms for SR, $11.2\pm9.34$ms for BiV, and $21.9\pm21.0$ms for RV. The mean absolute difference in activation times across all electrodes for ECGI is $5.81\pm4.65$ms for SR, $7.20\pm5.99$ms for BiV, and $6.99\pm5.11$ms for RV. The RMSE in predicted activation times is 18.9\% for SR, 24.4\% for BiV, and 31.6\% for RV. The RMSE of the predictions at each electrode is presented in Fig~\ref{fig:rmserealworldcombo}. The RMSE is consistently greater around the basal on the LV, apical on the RV and along the basel and mid-long axis on the septum. This may be due to the underlying heart-torso geometry which results in many similar BSPs for vastly different underlying HSPs. Future training sets may be bolstered with extra HSP-BSP pairs from these problem areas. 

\begin{figure*}[tbh]
\centering
  \includegraphics[width=\textwidth]{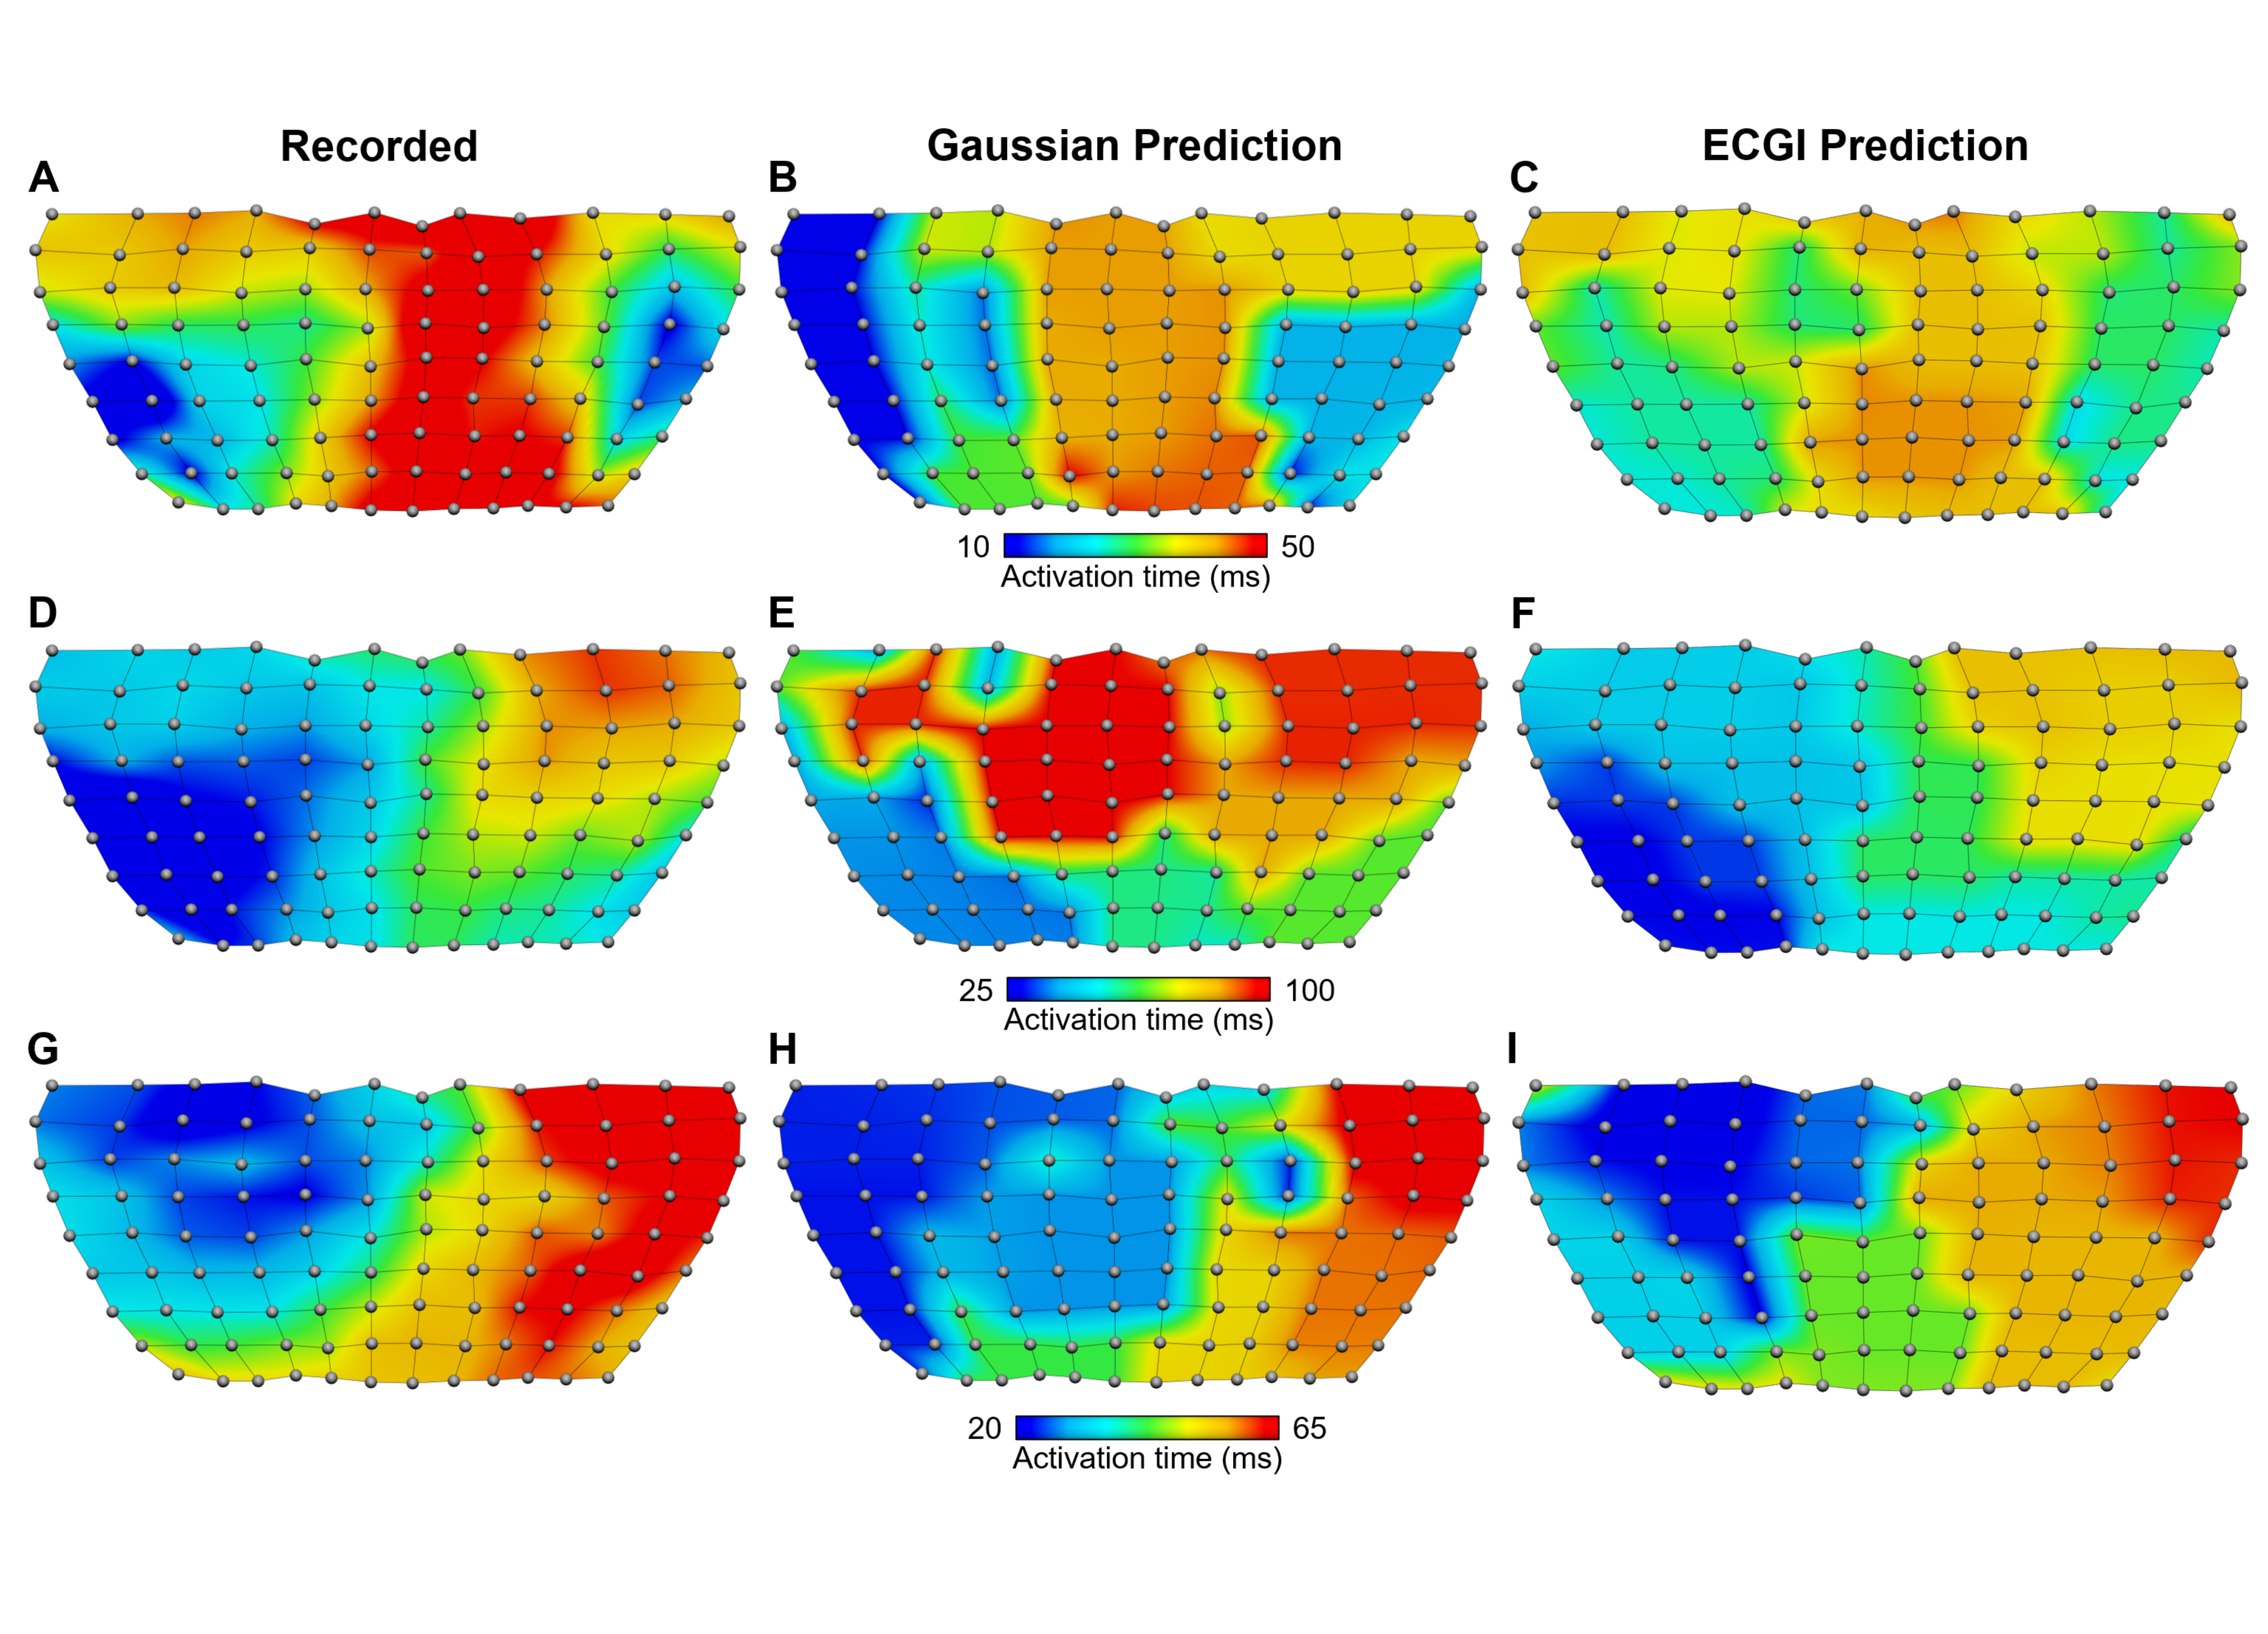}
  \caption{Comparisons between recorded and predicted heart surface activation and signals. A) Recorded activation sequence for bi-ventricular pacing. B) Impulse predicted activation sequence for bi-ventricular pacing. C) ECGI predicted activation sequence for bi-ventricular pacing  from~\mbox{\cite{Bear2018}}. D) Recorded activation sequence for right ventricular pacing. E) Impulse predicted activation sequence for right ventricular pacing. F) ECGI predicted activation sequence for right ventricular pacing from~\mbox{\cite{Bear2018}}. G) Recorded activation sequence for sinus rhythm pacing. H) Impulse predicted activation sequence for sinus rhythm pacing. I) ECGI predicted activation sequence for sinus rhythm pacing from~\mbox{\cite{Bear2018}}.}
  \label{fig:realworldothercombo}
\end{figure*}
\begin{figure*}[tbh]
\centering
  \includegraphics[width=0.66\textwidth]{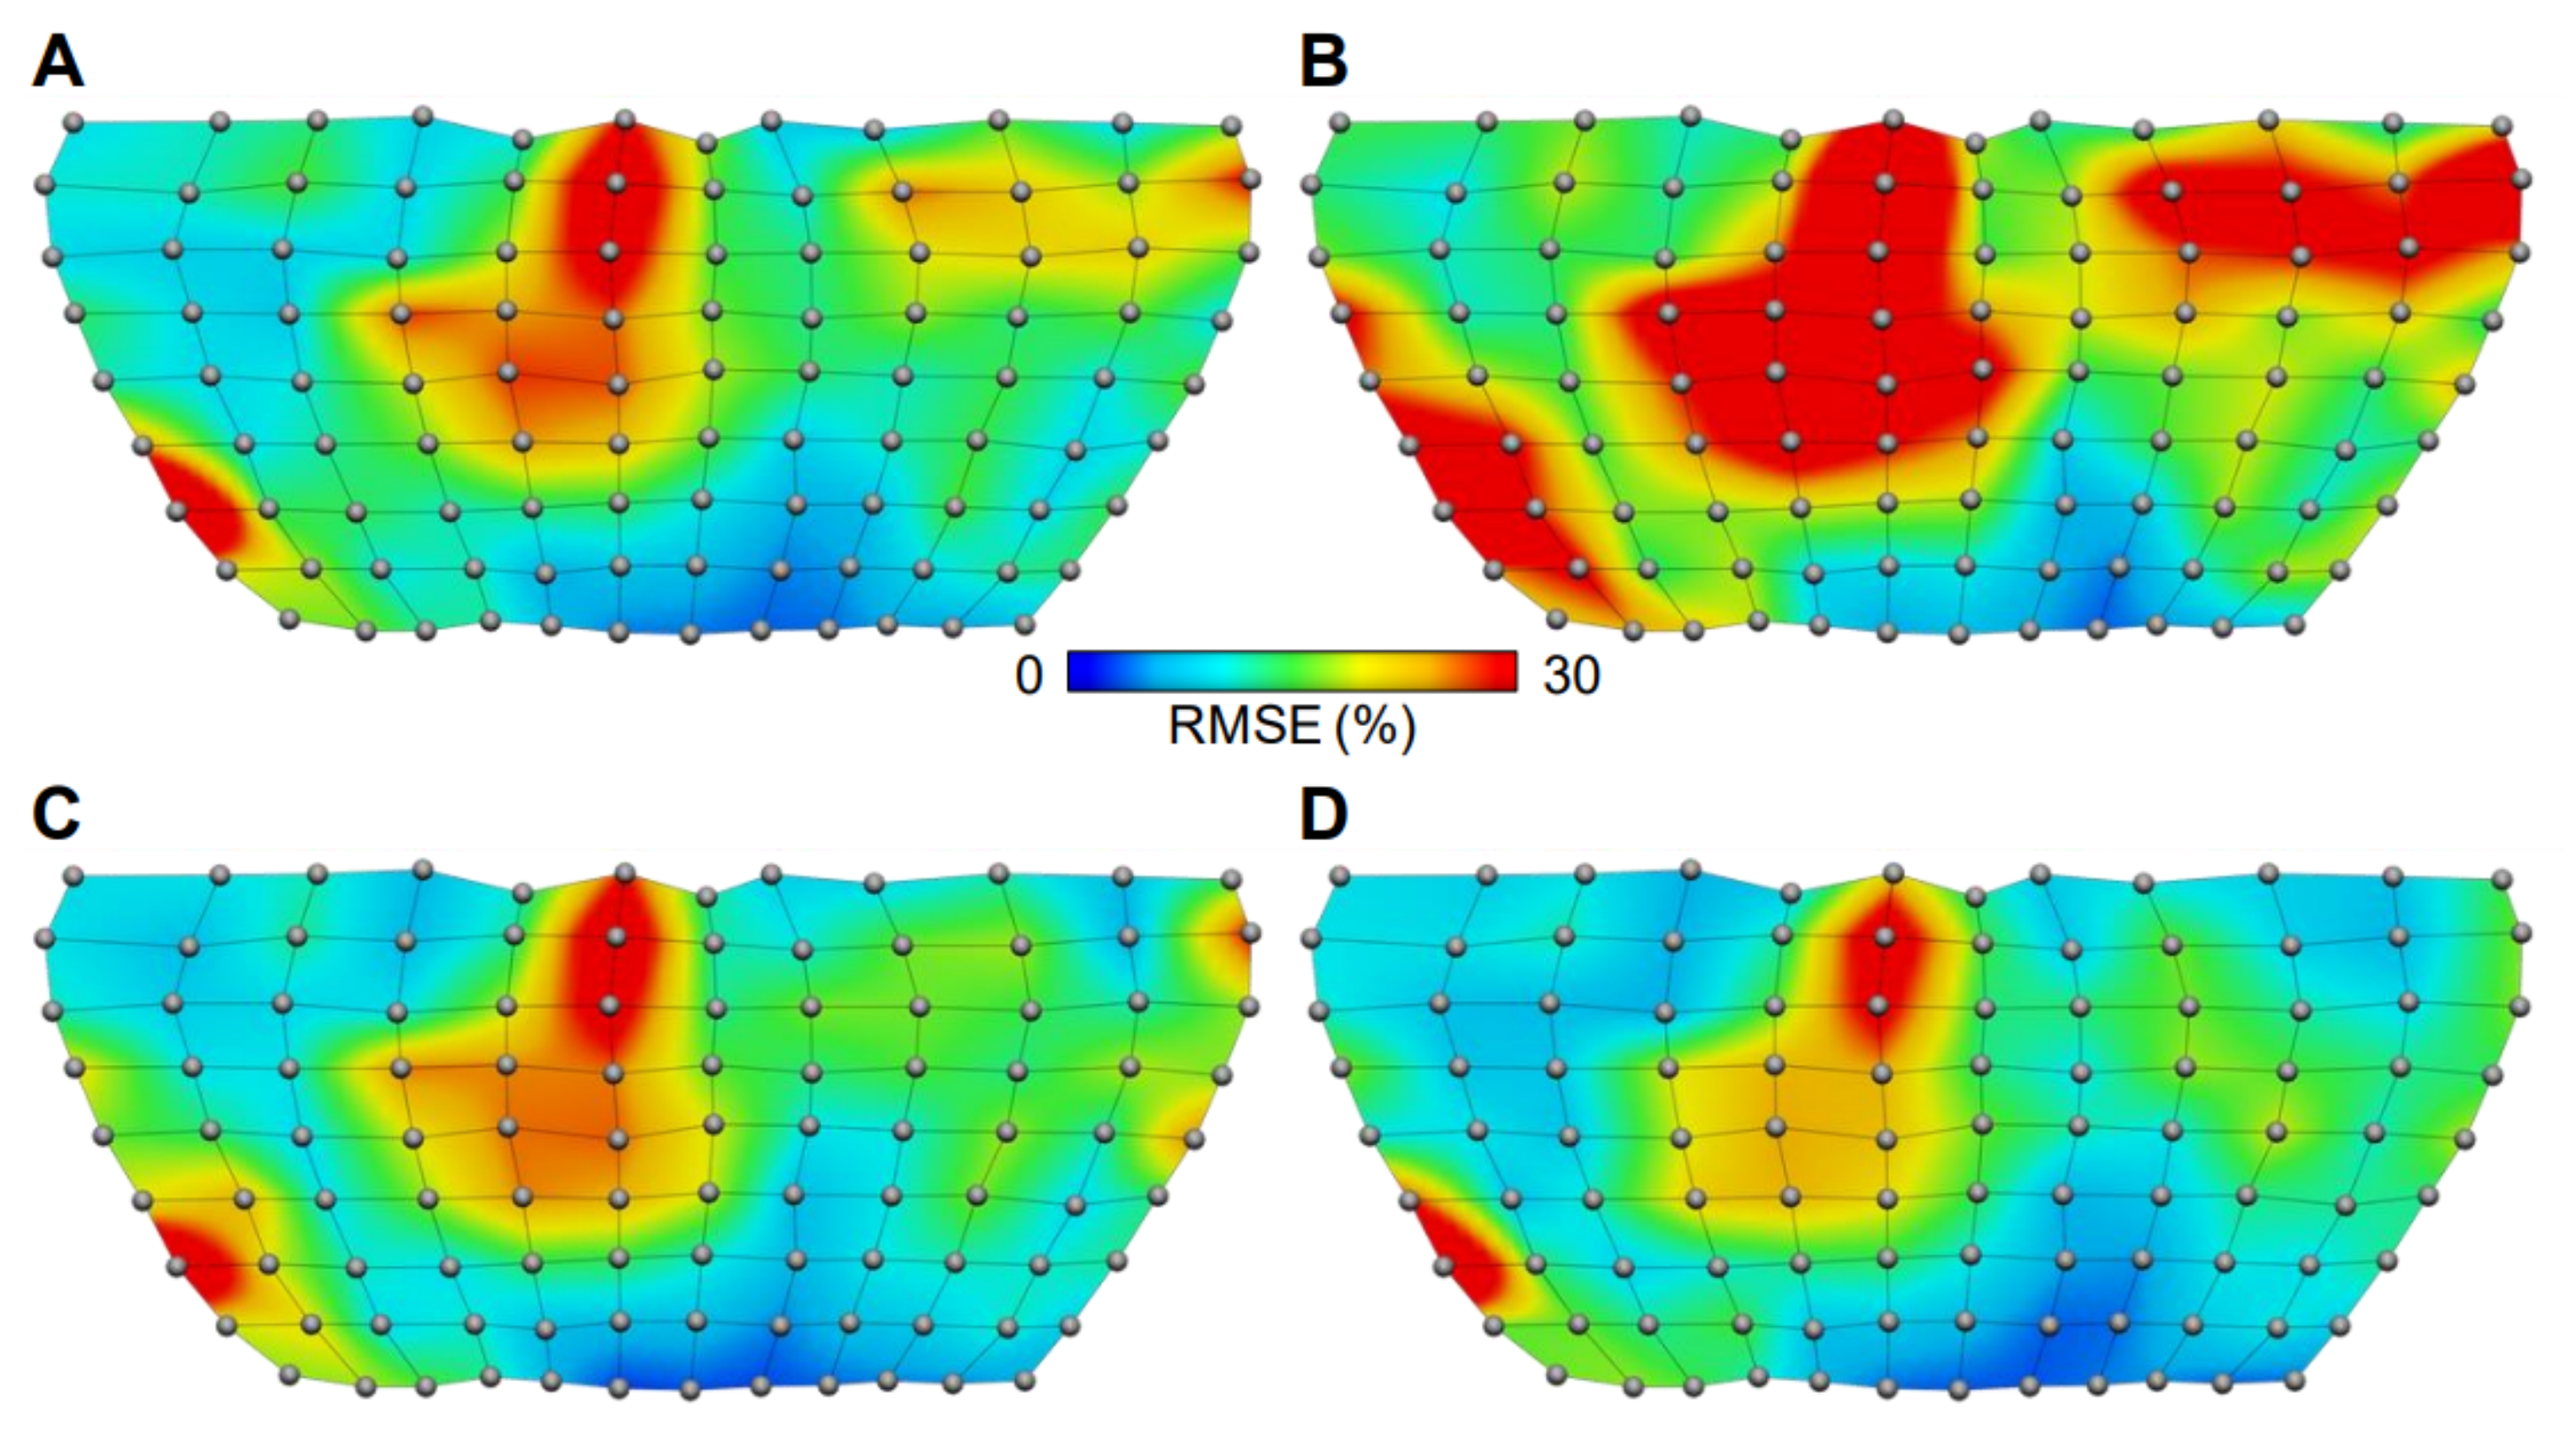}
  \caption{Root mean squared error (RMSE) between recorded and predicted heart surface signals at each electrode. A) Left ventricular pacing, B) Bi-ventricular pacing, C) Right ventricular pacing, D) Sinus rhythm.}
  \label{fig:rmserealworldcombo}
\end{figure*}
